# Supplementary material for: Deep Neural Compression Via Concurrent Pruning and Self-Distillation
Source: arXiv:2109.15014 source file (2021-09-30)
Supplement: Supplementary file 1 [file snr_additional.tex]

% This is often explicitly achieved in deep metric learning objectives using margin-based losses and contrastive losses maximize the similarity of positive pairs and minimize the similarity of negative pairs. Here, we posit that relative similarities between representations are encoded in the soft labels given by the teachers, producing similar dynamics to metric learned models. Moreover, they force the representations to have small intra-class distances and large inter-class distance. 

% Margin-based machine learning models maximize the boundary between classes during optimization, aiming to find a classification boundary that generalizes well on the test set. Intuitively, we expect SDP to implicitly force better separation between classes as we know from previous work \textbf{cite here} which finds self-distillation to do so. From this we can define a general scheme that measures the signal-to-noise ratio in $f^S$ as the means to understand how SDP may generalize better than magnitude-based pruning without self-distillation. 

%Let us define the SNR as $1/NC\sum_{i}^{N}\sum_{c=1}^{C}\frac{\mathbb{F}(\mat{Z}_c, \mathrm{shuffle}(\mat{Z}_c))}{\mathbb{F}}$
